# Supplementary material for: Rossby Wave Instability and Substructure Formation in 3D Non-Ideal MHD Wind-Launching Disks
Source: arXiv:2407.08032 source file (2024-08-14)
Supplement: Supplementary file 1 [file appendix_postprocess_dust.tex]

\subsection{method}
The post-process Lagrangian dust particles use similar methods as those in Tu 2019 and the tracer particles in Tu 2024. Lagrangian particles represent the dusts, and their equation of motion is given by
\begin{equation}
    \frac{d^2\mathbfit{x}}{dt^2} = \mathbfit{a}_\mathrm{gravity} + \mathbfit{a}_\mathrm{drag}
\end{equation}
where $\mathbfit{a}_\mathrm{gravity}$ is the acceleration due to gravity, and $\mathbfit{a}_\mathrm{drag}$ is the acceleration due to gas drag, given by
\begin{equation}
    \mathbfit{a}_\mathrm{drag} = \frac{\mathbfit{v}_\mathrm{gas} - \mathbfit{v}_\mathrm{dust}}{t_s}, \label{eq:pos_drag_force}
\end{equation}
where $\mathbfit{v}_\mathrm{gas}$ and $\mathbfit{v}_\mathrm{dust}$ are the local gas speed and instanteous dust speed respectively; $t_s$ is the stopping time of the dust particles in the Epstein regime \citep[e.g.][]{Epstein1924, Armitage15}
\begin{equation}
    t_s = \frac{\Tilde{\rho}_\mathrm{dm} s}{\rho_gv_\mathrm{th}}
\end{equation}
where $\Tilde{\rho}_\mathrm{dm}$ and $s$ are the dust material density and dust grain size respectively; $\rho_g$ and $v_\mathrm{th}=\sqrt{\frac{8k_bT}{\pi\mu m_H}}$ are gas density and gas thermal speed respectively. We take the mean-molecular-weight $\mu$ to be 2.33. The local gas quantities are obtained in the same way as Tu2024 and the equation of motion solver is also the same as in Tu2024.

When the dust particles are very small, $t_s$ can be so large that the solver is numerically unstable. To stabilize the simulation, we implement the ``small stopping-time approximation'': when the stopping time is less than the time-step of the simulation ($t_s < dt$), the dust velocity is approximated with
\begin{equation}
    \mathbfit{v}_d = (\mathbfit{v}_\mathrm{d, 0} - \mathbfit{v}_\mathrm{gas} - \mathbfit{a}_\mathrm{grav} t_s)\exp(-dt / t_s) + \mathbfit{v}_\mathrm{gas} + \mathbfit{a}_\mathrm{grav}t_s
\end{equation}
where $v_{d, 0}$ is the velocity of dust at the last time step, and the dust position is updated as
\begin{equation}
    \mathbfit{x} = \mathbfit{x}_0 + \mathbfit{v}_d dt
\end{equation}
where $\mathbfit{x}_0$ is the dust position at the last time step.

\subsection{comparision}
We present the comparison of the real Lagrange particles \citep[e.g.][]{Yang21, Hu22} and the post-procession dust scheme used in this paper. 
The post-procession dust scheme uses the quantities from the simulation output to represent unchanged background fields for each logical position corresponding to the simulation domain. 
Due to the dust in the post-process scheme not participating in the fluid evolution, the reduction of the cost for the numerical resource led to an achievement of a huge amount of post-processing dust input in the scheme. 

Fig. \ref{fig_live_vs_pos} shows the comparison of the scale height of the post-procession dust and the Lagrange particles. We accumulate the number of dust in the radius bins and calculate their standard deviation of the height to represent the dust scale height. 
The black line is the scale height of the post-procession dust function of radius, the red line is the scale height of the Lagrange particles, and the red dots represent the Lagrange particles. This test uses the standard conditions in the paper and fixes the grain size as 1mm. The distribution of the post-procession dust won't be the same as the real Lagrange particles; nevertheless, the scale heights of these two cases are not much different. 
\begin{figure}
    \centering
    \includegraphics[width=\linewidth]{Figures/scale_height_live_vs_pos_t00088.png}
    \caption{
    The comparison of the scale height of the post-procession dust and the Lagrange particles. The black line is the scale height of the post-procession dust function of radius, the red line is the scale height of the Lagrange particles, and the red dots represent the Lagrange particles. This test uses the standard conditions in the paper and fixes the grain size as 1mm.
    }
    \label{fig_live_vs_pos}
\end{figure}
